# Supplementary material for: Quantifying point cloud realism through adversarially learned latent representations
Source: arXiv:2109.11775 source file (2021-09-24)
Supplement: Supplementary file 1 [file experiments_anomaly_patch_noise.tex]

% !TEX root = ../paper.tex
%%
\begin{figure}
	\centering

	\begin{tabular}{lll}
		\textcolor{real_img}{\rule{2.4mm}{2.4mm}} \Real{} & \textcolor{syn_img}{\rule{2.4mm}{2.4mm}} \Syn{} & \textcolor{misc_img}{\rule{2.4mm}{2.4mm}} \Misc{}
	\end{tabular}

	\begin{subfigure}{0.48\linewidth}
		\centering

		\begin{tikzpicture}
			\begin{axis}[
				width=1.35\linewidth,
				enlargelimits=false,
				axis on top,
				axis equal image,
				ticks=none,
			]

			\addplot graphics[xmin=-60,xmax=60,ymin=-40,ymax=40] {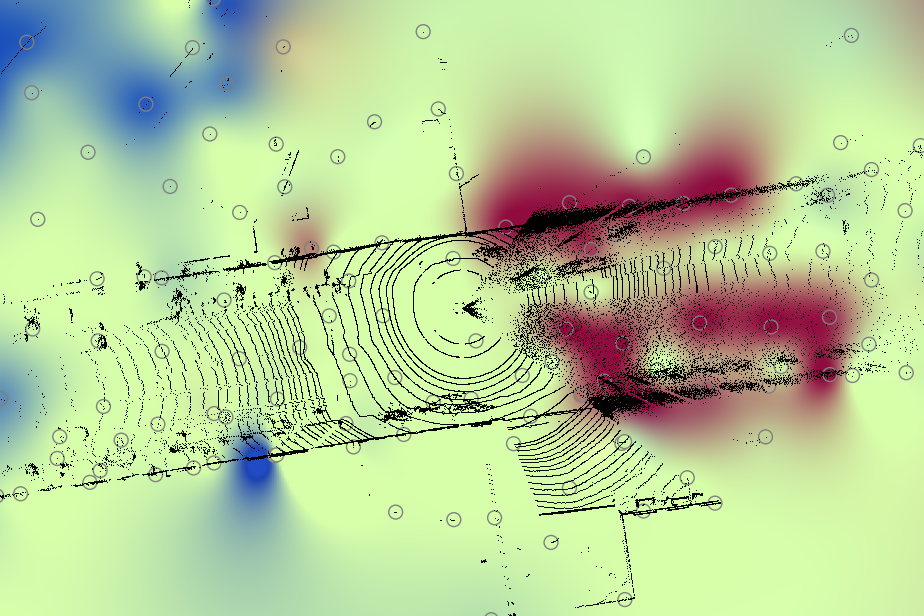};

			\draw[dashed] (0,0) -- (30,40);
			\draw[dashed] (0,0) -- (60,17);
			\draw[dashed] (0,0) -- (60,4);
			\draw[dashed] (0,0) -- (52,-40);

			\addplot graphics[xmin=-2.66,xmax=2.66,ymin=-1.4,ymax=1.4] {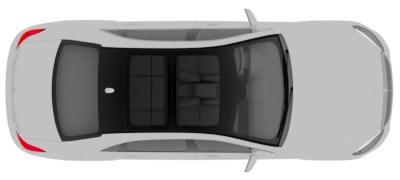};

			\end{axis}
		\end{tikzpicture}

		\caption{\label{fig:experiments_anomaly_patch_noise_low}Noise with $\sigma=1m$}
	\end{subfigure}%
	\hspace{4pt}%
	\begin{subfigure}{0.48\linewidth}
		\centering

		\begin{tikzpicture}
			\begin{axis}[
				width=1.35\linewidth,
				enlargelimits=false,
				axis on top,
				axis equal image,
				ticks=none,
			]

			\addplot graphics[xmin=-60,xmax=60,ymin=-40,ymax=40] {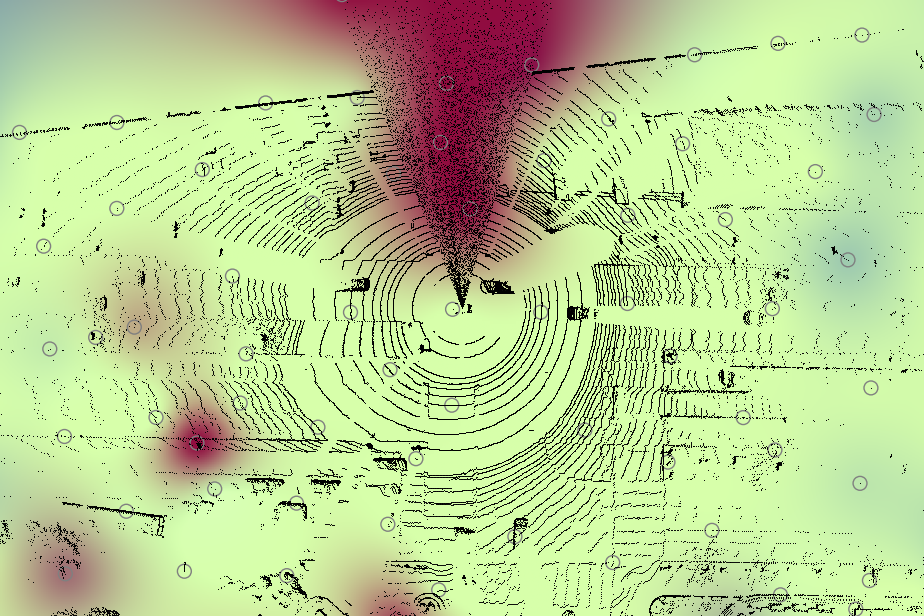};

			\draw[dashed] (0,0) -- (-16,40);
			\draw[dashed] (0,0) -- (12,40);

			\addplot graphics[xmin=-2.66,xmax=2.66,ymin=-1.4,ymax=1.4] {ego_vehicle_top_view_ortho.png};

			\end{axis}
		\end{tikzpicture}

		\caption{\label{fig:experiments_anomaly_patch_noise_high}Noise with $\sigma=8m$}
	\end{subfigure}

	\caption{
		\textbf{Detection of sensor failures}:
		Shown are two examples where randomly selected patches of PandaSet point clouds are distorted.
		Gaussian noise with standard deviation of $\sigma$ in meters is added to the original values.
		Shown are the interpolated softmax values for all three categories.
		The metric clearly identifies the regions with the distorted patches (purple regions).
		{\color{purple} TODO: can we make one figure with real-world anomalies to save space on the caption?}
	}

	\label{fig:experiments_anomaly_patch_noise}
\end{figure}
