# Supplementary material for: Quantifying point cloud realism through adversarially learned latent representations
Source: arXiv:2109.11775 source file (2021-09-24)
Supplement: Supplementary file 2 [file experiments_pandaset_gaussian_levels.tex]

% !TEX root = ../paper.tex
%%
\begin{figure}
    \centering

    \input{tikz/pandaset_gaussian_levels.tikz}

    \caption{
        \textbf{Gaussian Distortion Levels}:
        The x-axis shows increasing values of Gaussian noise that is applied to the distance measurements of PandaSet point clouds.
        When the noise factor increases, the \Real{} score declines while the Misc score rises.
        For small standard deviations the data appears slightly more synthetic, therefore the Syn score increases slightly before declining at higher noise levels.
    }
    \label{fig:experiments_distortion_levels}

\end{figure}
