# Supplementary material for: Quantifying point cloud realism through adversarially learned latent representations
Source: arXiv:2109.11775 source file (2021-09-24)
Supplement: Supplementary file 3 [file experiments_upsampling_metric_2x.tex]

% !TEX root = ../paper.tex
%%
\begin{table}
	\centering

	\caption{
		\textbf{Metric Scores over Up-Sampling Methods}:
		This table compares five different up-sampling method and displays the \textit{Ground Truth} scores for reference.
		Here, 2~$\times$~resolution enhancement was conducted.
		We report three classical metric scores, Mean Squared Error (MSE), Mean Absolute Error (MAE), and Chamfer Distance (CD).
		These scores show the reconstruction errors between the up-sampled data and the \textit{Ground Truth} target.
		The other three scores, Misc, Real and Syn, are the mean softmax results of our metric which does not require a target.
	}

	\label{tab:experiments_upsampling_metric_2x}

	\resizebox{\linewidth}{!}{%
	\begin{tabularx}{\linewidth}{lrrrrrr}
		\toprule
		\makecell[l]{Up-Sampling\\Method} & MSE & MAE & CD & Misc & Real & Syn \\
		\midrule
		Ground Truth			& 0.00 & 0.00 &   0.0 & 0.02 & 0.69 & 0.29 \\
		Nearest Neighbor		& 0.38 & 1.83 & 122.0 & 0.01 & 0.65 & 0.34 \\
		Bilinear				& 0.88 & 0.15 &  75.2 & 0.03 & 0.65 & 0.32 \\
		$\mathcal{L}_1$-CNN	& 0.37 & 0.59 &  16.7 & 0.05 & 0.66 & 0.30 \\
		$\mathcal{L}_2$-CNN	& 0.56 & 0.69 &  16.7 & 0.13 & 0.58 & 0.29 \\
		GAN					& 0.93 & 1.46 &  76.9 & 0.16 & 0.56 & 0.28 \\
		\bottomrule
	\end{tabularx}
	}  % end of resize box

\end{table}
